# Supplementary material for: Task-Oriented Active Learning of Model Preconditions for Inaccurate Dynamics Models
Source: arXiv:2401.04007 source file (2024-04-23)
Supplement: Supplementary file 1 [file supplementary.tex]

\clearpage
\appendix                                 
\begin{center}
    \huge{Appendix}
\end{center}

\section{GP Implementation Details}

The aleatoric noise in the model deviation in a more complex problem varies in $\mathcal{S} \times \mathcal{A}$, which we account for with a heteroscedastic noise model. 

We use a standard GP regression model with a Matern kernel with the addition of a noise model that captures the heteroscedasticity of the data. We will assume that the variance of the noise term $\epsilon_i$ at each data point $x_i$ is a function of the input features $x_i$, i.e., $\epsilon_i = \sigma(x_i)^2$. The noise function $\sigma(x_i)$ will be modeled using a separate GP that takes the input features $x_i$ as input. We approximate the observation by cross-validating subsets of $\epsilon_i$ using a homoscedastic model, and then using that to fit the heteroscedastic noise model. 

We use the BoTorch implementation of a GP regression model with a gpytorch backend but optimize the hyperparameters by alternating optimization using BoTorch for 5 iterations for training step and marginal log-likelihood at each training iteration~\cite{balandat2020botorch}. We needed to set lower and upper bounds on the kernel lengthscales for both the noise model and for the homoskedastic. 
\ed{Additionally, due to space limits for using an exact GP, we randomly sampled a subset of 300 points from the full set of training data.} 
\section{Additional Details on Experimental Scenarios}
\subsection{Slippery Grid World}
\label{ref:detailsgridworld}
The state in the grid world is a two-dimensional $(x,y)$ environment. The robot can move up, down, left and right. It cannot move through walls, and moving left or right across the ``slippery'' squares causes it to move backwards by one step. This is the same environment as was used in ~\cite{vemula2020planning}.
\subsubsection{Dynamics Model}
\label{ref:gridworlddynamicsmodel}
\ed{The dynamics model for the Grid World is: $\uparrow$ (up) increases $y$ by 1, $\downarrow$ (down) decreases $y$ by 1, $\leftarrow$ (left) decreases $x$ by 1, and $\rightarrow$(right) increases $x$ by 1. If the next location is outside the bounds of the grid, the dynamics model assumes that the robot stays in place. The dynamics model does not account for the ``slippery'' squares however. }
\subsection{Simulated Plant-Watering}
\ed{The state is represented as $x,y,\theta$. In the target environment, a plant is constructed out of voxels to mimic a Monstera plant.  Water can pass through holes in the top of the leaves, but not through solid sections.}
\subsubsection{Dynamics Model}
\ed{This is the only task where we use a learned model. The learned model was trained on a variation (meaning only one randomly selected geometry) of the \texttt{PourWater} Softgym~\cite{lin2021softgym} environment, which does not contain a plant. 7 actions are sampled (some with $\theta_d = 0$ and some randomly sampled between $\theta_d \in [1,3]$) and executed to form a dataset of 1200 trajectories or 8400 transitions. 10\% were held out as a validation set. }

\ed{The model was trained using the Adam optimizer with a learning rate of 0.004 with a batch size of 64, $128 \times 128 \times 128$ fully connected layers with Dropout and ReLU activation. Training was ended after 300 epochs, which is when the validation loss reached an accuracy corresponding to approximately 1 cm of position error, and 10\% volume accuracy. }

\ed{Because there is no plant in the dataset that the model was trained on, the predictions overestimate the amount of water in the target container for pouring actions above the leaves, and in actions that interact with the leaves (potentially leading to the controlled container not being able to move to the desired pose).}

\label{ref:simdynamicsmodel}
\label{ref:detailssimworld}
\subsection{Real-world Plant-Watering}
\label{sec:hardwarepouring}

The experimental setup is shown in Figure~\ref{fig:experimentalsetup}. We use a Franka Emika Panda robot. To protect the robot from water that splashes out of the container, we cover it in the Fluid Resistant Cover from Robo-Gear. Outside equipment is protected using Vention bars surrounded by polycarbonate with a slideable door. 
%the design for which can be found \href{https://cad.onshape.com/documents/cd60b8dd737026b1df6dfa47/w/1076f2e96e64906b0ff8f1b7/e/26ebf60c20c7a7ade6d438d6?renderMode=0&uiState=643af1662ba9ed2cb5416e35}{at this link}. 
The base of the environment is covered in highly absorbent PIG Mat in 15-inch by 20-inch squares that absorb 14 oz of water each. Resets are performed by pouring out water in the plant container, replacing wet mat with a dry mat, or waiting for the water to evaporate. 

\begin{figure}[h]
\centering
\includegraphics[width=0.8\textwidth]{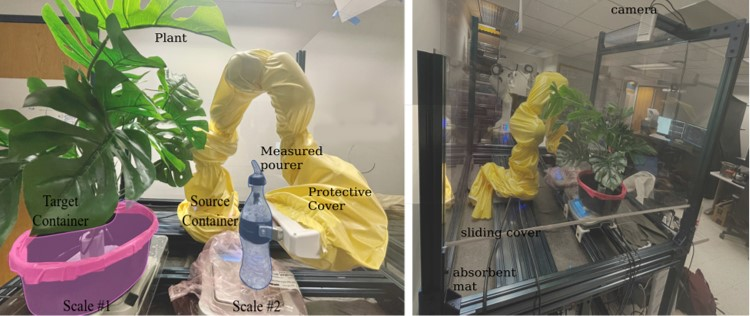}
\caption{Two annotated views with the components of our real-robot pouring setup designed to allow the robot to spill small amounts of water into the workspace without damage.}
\label{fig:experimentalsetup}
\end{figure}

The state is represented as the poses of all containers containing water and their volumes. The target container pose is fixed at $x_{target}, y_{target}, z_{target}$. The pose of the source container is $x_{source}, y_{source}, z_{source}$ and contains an orientation parameter representing the rotation about the z-axis: $\theta_{source}$. The volume of the source and target container respectively are $v_{source}$ and $v_{target}$. Actions are defined as target locations for $y_{source}, z_{source}, \theta_{source}$. The desired location is denoted as $y_d, z_d, \theta_d$. $x_d$ is fixed to a single value to keep motion in one plane. Trajectories are defined for the controlled container, but the motions are generated kinematically using the grasp transform between the bottle and the end-effector. There are broad preconditions for the actions, but do not specify where the model will be accurate. For example, $y_d, z_d$ cannot be in collision with the target container. If $\theta_{target} > 1$ , then $y_d$ and $z_d$ must be equal to $(y_{source}, z_{source})$, and $y_d, z_d$ must be within a fixed distance of $y_{target}, z_{target}$ .
\subsubsection{Dynamics Model}
\ed{The dynamics model for real-world watering is an idealized analytical model. The reason we can specify this is because the robot was pouring with a measured pourer, which dispenses 17 mL. A flowchart shown in Figure~\ref{fig:realworldanalyticalflowchart} shows the logic for the analytical model that we use. }

It is  ``idealized'' in that it assumes:
\begin{enumerate}
\item The robot always reaches the desired container position
\item 17 mL \footnote{Although we were using a 15 mL measured pourer, we found that 17 mL was typically poured from it in practice, so we actually used  } always leaves the container when poured greater than 130 degrees
\item 17 mL enters the target container if the location of the controled container is above the area of the target container 
\end{enumerate}

\begin{figure}
\edfigure{
\includegraphics[width=0.5\textwidth]
{imgs/idealizedanalyticalflowchart.pdf}
}
\caption{\ed{Flowchart illustrating the analytical model used for pouring in the real world}}
\label{fig:realworldanalyticalflowchart}
\end{figure}

\subsubsection{State estimation}
\ed{In this scenario, the state of the plant is represented only by the pose of the target container and assumed to be fixed relative to the target container. The target container has a bright pink rim and is measured using an overhead Azure Kinect DK camera. The target container is detected in the image by using the OpenCV circle detector and color thresholding. The pixels inside the circle (after filtering out pixels that belong the plant) are converted to a pose by using the camera intrinsics, which are then deprojected into camera frame. The camera frame is calibrated extrinsically to world frame, so the pose of the target container is known in world frame.  In many configurations, the leaves obstruct the tape, in which case we use the last measured pose. }

\ed{The state of the container is observed indirectly using the proprioception of the robot, assuming a fixed transform between the container and robot, and two  U.S. Solid Precision Laboratory 3000 g High Precision Analytical Balances are used for measuring the weight of the water. The scales are not reset between trajectories, so the volume of the target container typically increases as more data is collected, and the measured volume of the bottle decreases as more data is collected.}

\subsubsection{Minimizing Human Intervention in Data Collection}
\ed{Many design decisions in this environment were made to reduce the need for human intervention in the data collection procedure, which we describe here. At the beginning of data collection, the water bottle needs to be filled and the walls to the environment lowered to prevent splash damage to electronic components. Scales are tared programmatically through the serial interface and do not need to be touched. At the beginning of a trajectory, the robot measures the state of the scene, including the water volume of each container. It uses the same fixed side grasp to grasp the central part of the water bottle. Planning and trajectory execution are all autonomous. Once the trajectory for data collection or evaluation is executed, the robot returns the water bottle to the scale by placing it down, and then moves above the scale to enable an accurate measurement. }

\ed{Despite our attempts to minimize human supervision, there were a few cases where a human needed to occasionally intervene (about one in fifteen trajectories). The most common one is if the bottle slips or is placed in an unstable configuration, which happened sometimes when the bottle was close to empty. Such conditions can be remedied by using a bottle with a more stable base. The second case where human intervention was necessary was if the plant fell due the robot getting stuck in the leaves, which occurred rarely. }

\ed{All state estimation, including detecting whether the desired volume of water was in the target container, and whether a significant portion was spilled, is done autonomously. }

\subsubsection{Joint-Space Trajectory Execution}
\ed{The paths from planning are represented as controlled container poses and the trajectories are generated to follow that path. The desired end-effector poses can be obtained straightforwardly by applying the inverse grasp transform to the desired controlled container poses. For motions where $\theta_d=0$, a joint-space trajectory is generated with 10 waypoints, using an IK solver to convert the poses to joint configurations. The same joint-space trajectory generation process is followed for actions where $\theta_d > 0$, which results in the pouring motion as the bottle changes angle. }

\ed{In this environment, we found that a simple IK solver would frequently find solutions where the robot was in self-collision, or in collision with obstacles. Rejection sampling was insufficient to avoid these solutions, but we were able to find solutions using the PyTorch Robot Kinematics library~\cite{Zhong_PyTorch_Kinematics_2023}, which accounts for collisions in the solver. }

To follow the joint-space trajectories, we use the joint position controller from \cite{zhang2020modular}.

\subsection{Motion Planning Implementation}
\label{sec:motionplanning}
\ed{Problems are described in terms of their low-level state space. We use an RRT planner in a fairly standard manner: sample a random state, and then add actions to the tree that move toward that state. The predicted results of the actions are computed using the forward dynamics model, $s' \gets \hat{f}(s,a)$. $s'$ is added to the tree if the edge toward it does not violate the constraints. The constraints are that the original $(s,a)$ are within the model precondition of $\hat{f}$, and that $s'$ does not have collisions. Collision checking is implemented using pybullet through the PyBullet planning library~\cite{pybulletPlanning} for the real-world scenario, and using Flexible Collision Library~\cite{pan2012fcl} for the simulated scenario. There are no constraints in the GridWorld problem.} 

\ed{We use the Open Motion Planning Library implementation of RRT~\cite{sucan2012open} for its speed and popularity. The planner can perform up to 5000 expansions before it times out, except during the online learning phase, where the planner times out after 30 seconds.  }

\section{Additional Qualitative Analysis of MDEs over Online Learning Runs}
\ed{In this section, we look at plot model preconditions and acquisition function values in the simulated watering environment for individual online learning runs. First, we analyze the step-wise acquisition function values to better understand the relative utility of points in space during training based on the MDE estimates. Then, we look at the corresponding model preconditions defined by the MDE learned during training. More quantitative data of the types of trajectories chosen across all seeds can be found in Figure~\ref{fig:trajtypes}. }

\ed{Because the MDEs are defined over a five-dimensional space in this settings, in order to view a 2D cross section, we vary $x_{source},y_{source}$ and $x_d, y_d$ for a fixed $\theta_d$ that is the median $\theta_d$ observed for actions that result in all the water ending up in the target container. $x_d=x_{source}$ and $y_d=y_{source}$, which is close to in-distribution for the training data, where actions either have a significant change in angle or position but not both. }

\subsection{Illustrative Example: Successful Balance of Exploration and Exploitation}
\label{sec:illustrativeexamplesuccess}
 that demonstrated good performance. 
\ed{Figure~\ref{fig:goodsimacqexample} shows an example of acquisition function values and the distribution of training points. In Iteration 2, we observe that the algorithm collects points with high error from unsuccessful high pours, corresponding to the higher number of \texttt{above\_spill} pours at the beginning of training. By iteration 5, there are enough high-error pours above the leaves such that the region becomes red (low-utility) due to a low $\mu(s,a)$ for those states. This corresponds to the general decrease in \texttt{above\_spill} pours.  The best acquisition function value regions are in either unknown unreachable locations above the plant, or in the now darker shaded (lower and better value) region under the plant leaves. Higher values where $\sigma$ is higher leads to more data collection at regions near the edge of the box. There is a slight drop in \texttt{below\_success}-type trajectories about halfway through training as more samples from the uncertain (high $\sigma$) region are collected. By iteration 15, the edge of the region where the model is accurate shows higher $\mu$ and lower $\sigma$. }

\ed{The corresponding model preconditions are shown in Figure~\ref{fig:goodsimprecondexample}. In iteration 2, there is a clear lower deviation region under the leaves, but not sufficient to confidently find plans where $\hat{d}(s,a) < \dmax$ with high enough probability when $\beta=2$. The area above the plant is predicted high deviation. As desired, the region where $\hat{d}(s,a) < \dmax$ increases in size from iteration 5 to 15, reflecting a higher success rate in computing plans to the goal in later iterations.}
\begin{figure}
    \centering
    \begin{subfigure}[b]{\textwidth}
    \edfigure{
    \includegraphics[width=\textwidth]{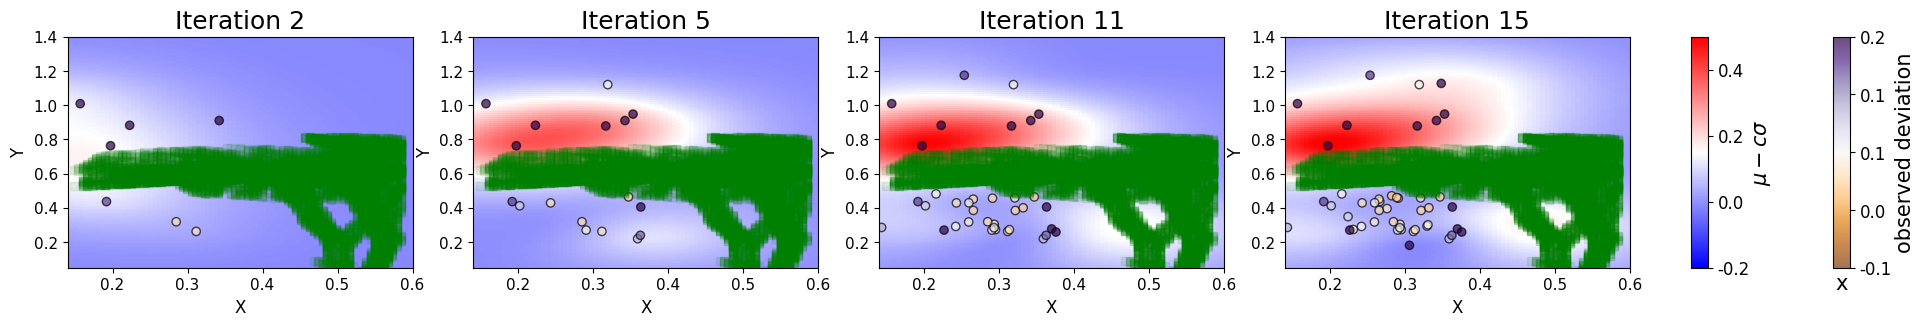}}
    \caption{\ed{Step-wise acquisition function values, $\alpha_{step}(s,a)$ over online learning iterations for actions where $\theta_d > 130$ degrees over $x_d$ and $y_d$, shown using the color bar on the right. The shading of the a dot indicates the ground-truth deviation of an observed sample. The shading of the region shows the acquisition function value, where the lower the value, the higher utility the point is. A cross-section of the plant is shown for reference.}}
    \label{fig:goodsimacqexample}
    \end{subfigure}
    \begin{subfigure}[b]{\textwidth}
    \edfigure{
    \includegraphics[width=\textwidth]{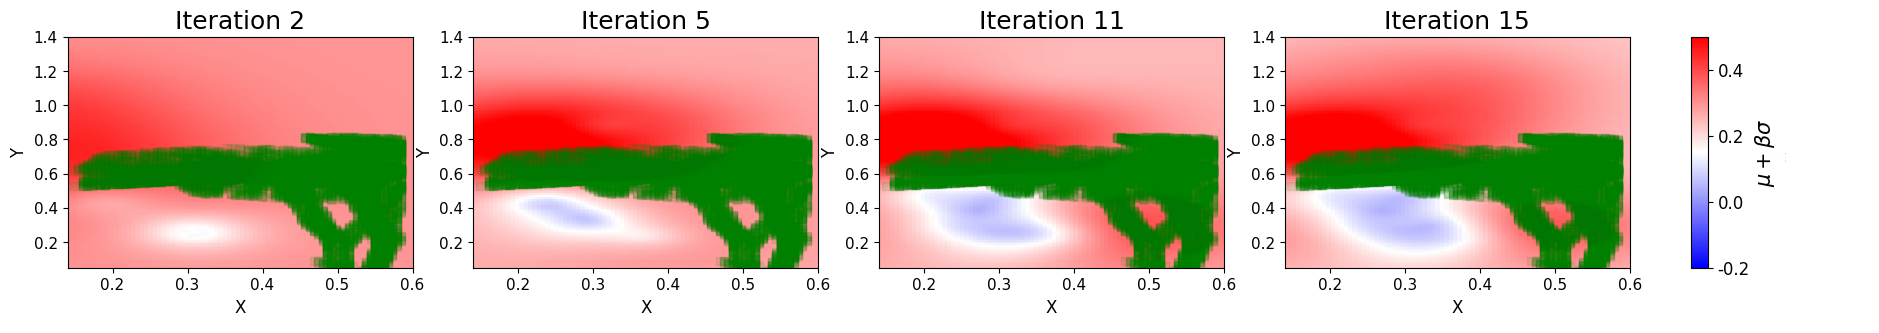}}
    \caption{\ed{MDE values over online learning iterations for actions where $\theta_d > 130$ degrees over $x_d$ and $y_d$, shown using the color bar on the right. The shading of the region shows the MDE value where white indicates $\dmax$ for this setting. $\beta=2.0$  A cross-section of the plant is shown for reference.}}
    \label{fig:goodsimprecondexample}
    \end{subfigure}
    \caption{Example of desired behavior in active learning run}
\end{figure}
\subsection{Illustrative Example: Failing to Find Sufficient Model Precondition}
\label{sec:illustrativeexamplefailure}
\ed{In this section, we analyze a failure case: an individual run where the robot is unable to reliably compute plans to solve the task within the time limit. The resulting model precondition is in Figure~\ref{fig:badsimprecondexample}. The region that is blue (below $\dmax$) is much smaller compared to the model precondition in Figure~\ref{fig:goodsimprecondexample}. Additionally, the points are in a more constrained part of the environment, right below the leaves. The smaller precondition is explained by the data observed, especially samples that cause a high noise estimate in that region. There is a particularly interesting phenomemon where $\alpha_{step}(s,a)$ values are particularly low in a noisy region where high-deviation samples are observed in close proximity to low-deviation samples. Such noise increases $\sigma$ due to aleatoric (rather than epistemic) uncertainty, leading to two  results that cause a low success rate in finding plans. First, the acquisition function biases the robot to collect data in noisier parts of the space even though aleatoric uncertainty typically does not reduce with more data the way epistemic uncertainty does. Second, those noisy parts of the space are excluded from the model precondition. Points that are $y_{source} < 0.25$ are not explored in this run although they were collected in the run shown in Figure~\ref{fig:goodsimacqexample}.}

\begin{figure}
    \centering
    \begin{subfigure}[b]{\textwidth}
    \edfigure{
    \includegraphics[width=\textwidth]{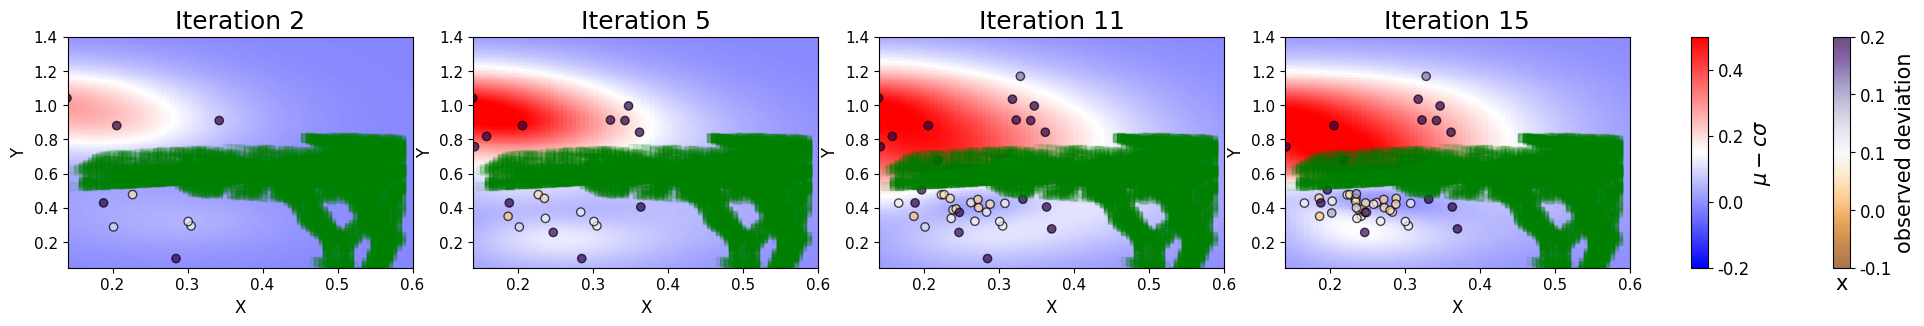}}
    \caption{\ed{Step-wise acquisition function values, $\alpha_{step}(s,a)$ over online learning iterations for actions where $\theta_d > 130$ degrees over $x_d$ and $y_d$, shown using the color bar on the right. The shading of the a dot indicates the ground-truth deviation of an observed sample. The shading of the region shows the acquisition function value, where the lower the value, the higher utility the point is. A cross-section of the plant is shown for reference.}}
    \label{fig:badsimacqexample}
    \end{subfigure}
    \begin{subfigure}[b]{\textwidth}
    \edfigure{
    \includegraphics[width=\textwidth]{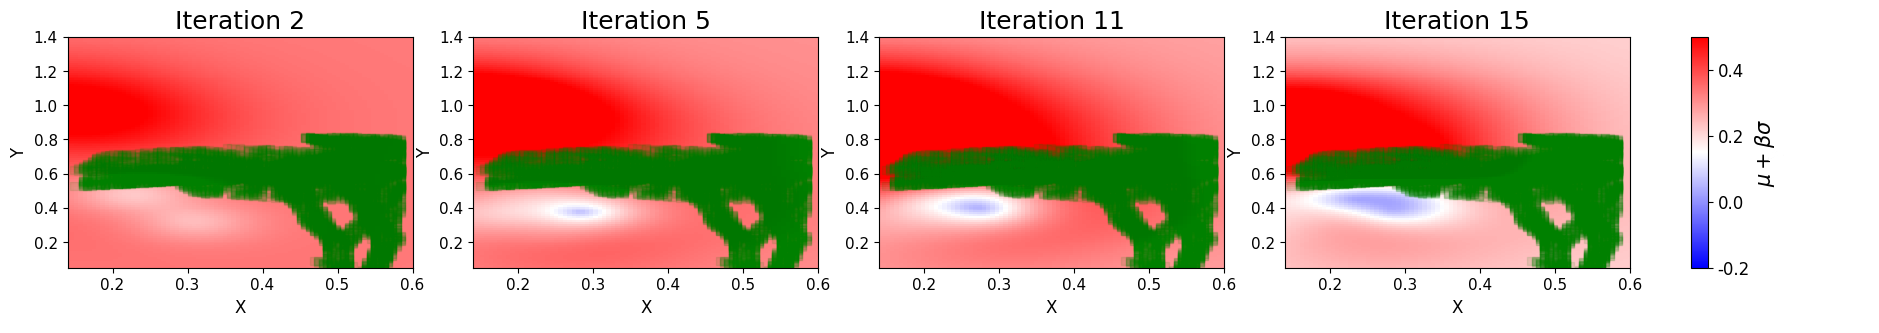}}
    \caption{\ed{MDE values over online learning iterations for actions where $\theta_d > 130$ degrees over $x_d$ and $y_d$, shown using the color bar on the right. The shading of the region shows the MDE value where white indicates $\dmax$ for this setting. $\beta=2.0$  A cross-section of the plant is shown for reference.}}
    \label{fig:badsimprecondexample}
    \caption{Example of undesired behavior in active learning run}
    \end{subfigure}
\end{figure}

\section{Additional Results for Active Learning Quantitative Analysis}
\label{sec:additionalresults}
\subsection{Trajectory diversity}
In the next experiment, we evaluated the effect of enforcing a diverse trajectory set on performance by enforcing that the candidates in $\bm{\mathcal{T}}$ are different from each other. In default \ab, we enforce trajectory diversity. For this experiment scenario, we bin the heights that each candidate trajectory can end at to enforce different types of trajectories. The no-bins version removes this mechanism, so the only randomness in the trajectories comes from RRT. Our results are shown in Figure~\ref{fig:trajdiversity}.
\begin{figure}[h]
\centering
    \begin{subfigure}{\plotwidth}
        \includegraphics[width=\textwidth]{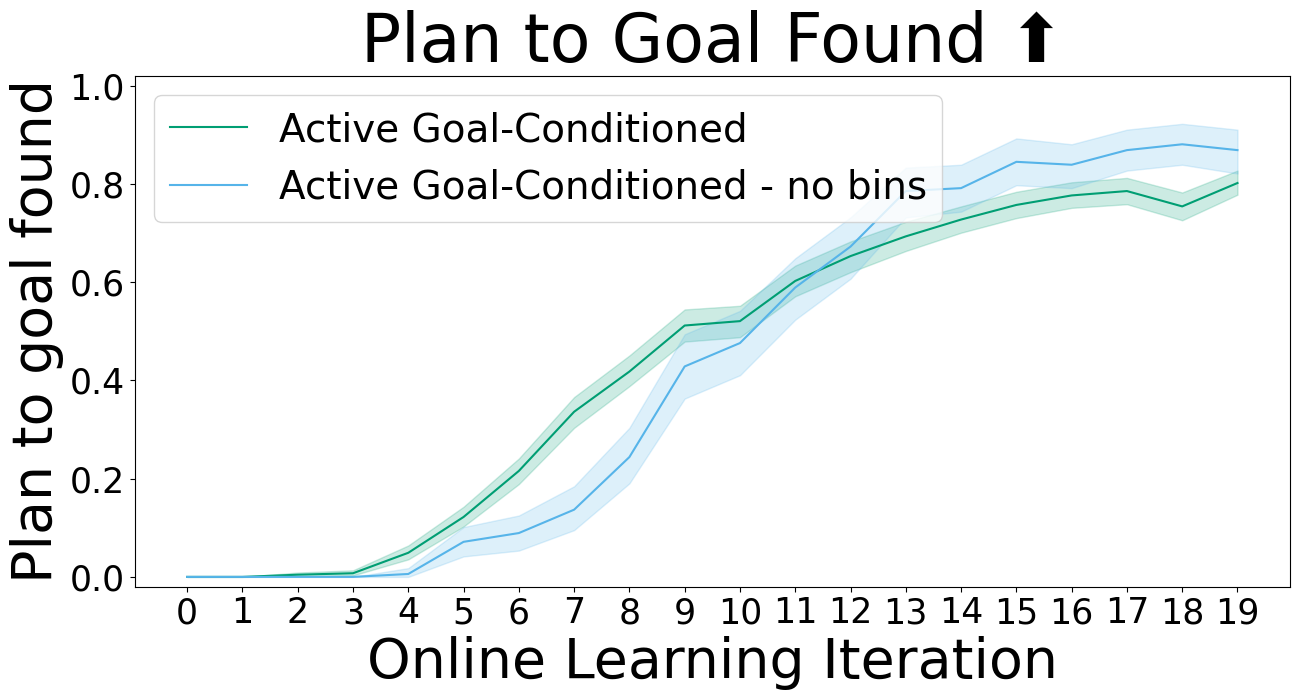} 
    \end{subfigure}
    \begin{subfigure}{\plotwidth}
        \includegraphics[width=\textwidth]{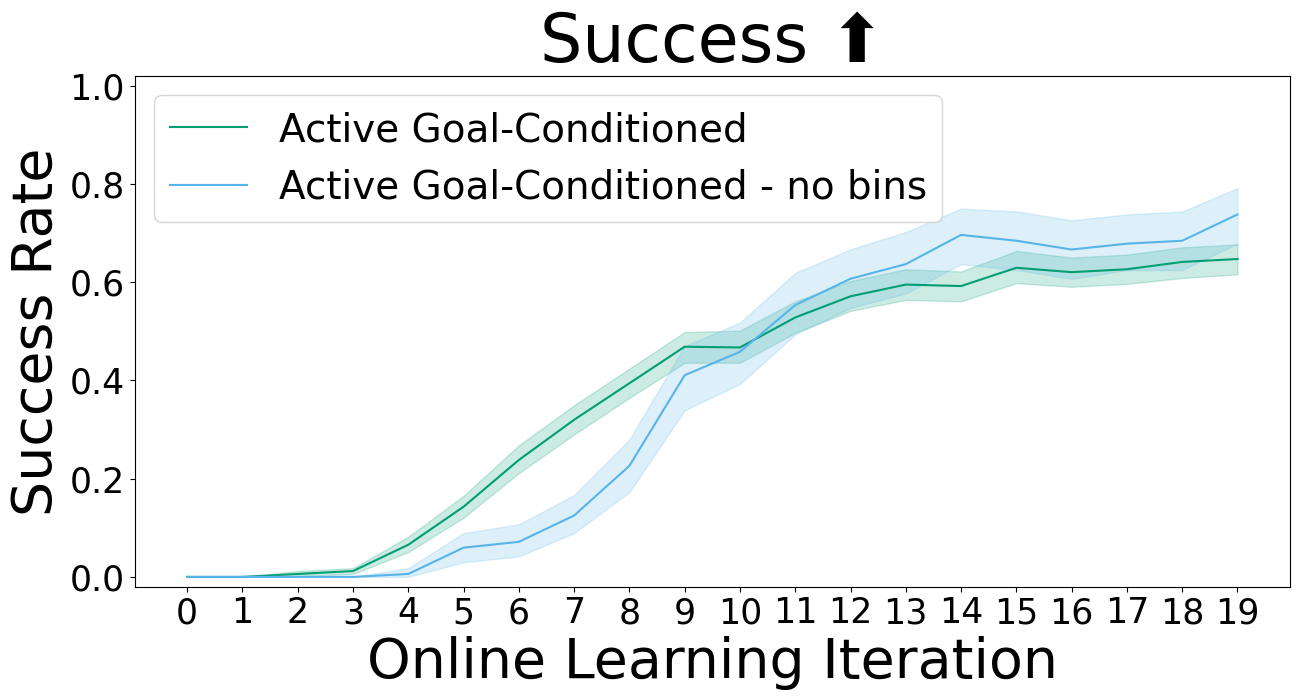} 
    \end{subfigure}
    \begin{subfigure}{\plotwidth}
        \includegraphics[width=\textwidth]{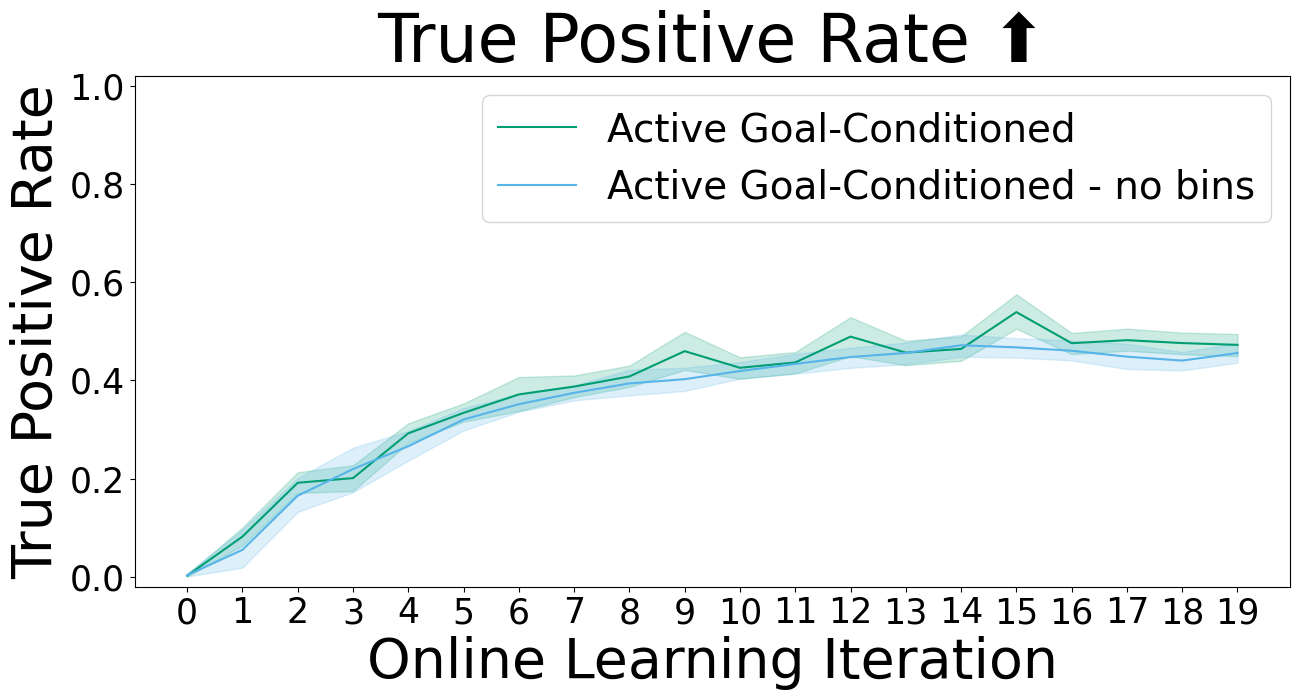} 
    \end{subfigure}
    \begin{subfigure}{\plotwidth}
        \includegraphics[width=\textwidth]{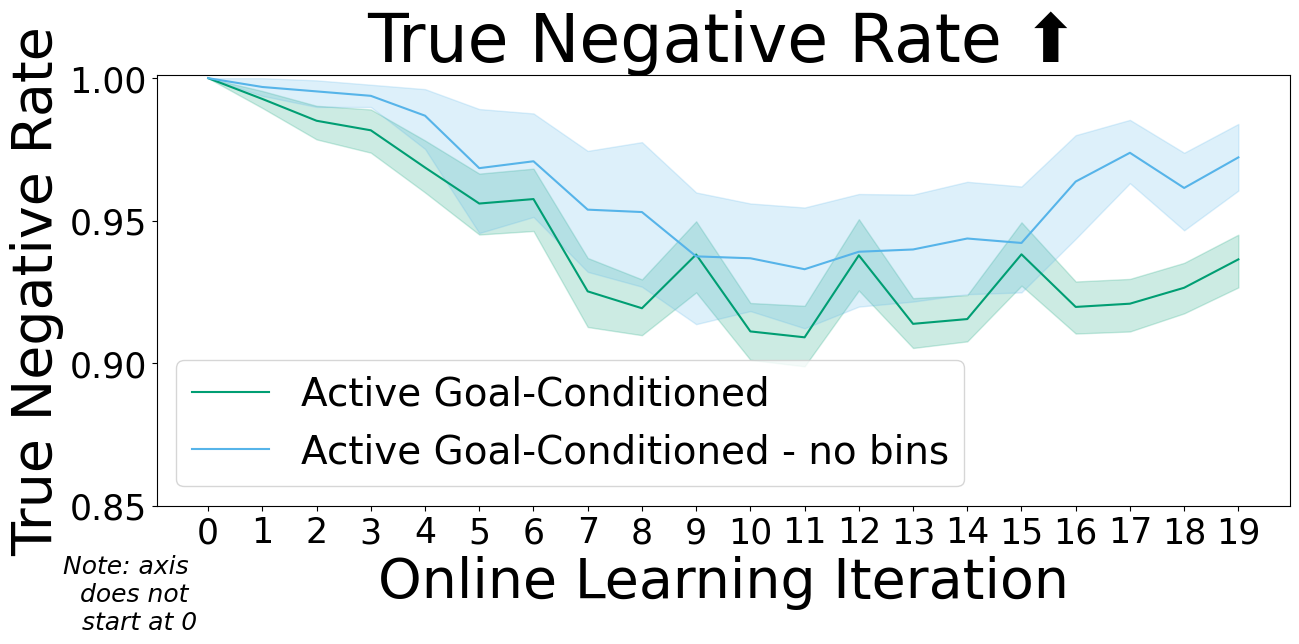} 
    \end{subfigure}
\caption{Effect of artificially enforcing trajectory diversity  on active learning performance}
\label{fig:trajdiversity}
\end{figure}

We find some improvement in performance with less data when using the binning to increase diversity. However, the ability of the planner to find plans improves in later iterations with binning removed, which may be due to a better match of the states visited during planning, since binning is not used after active learning. The \tnr is better for the version without bins with more data, the \tpr is similar, but the version that does not use bins has a higher success rate in finding plans to the goal. 

Additionally, the good performance of the version with no bins indicates that the binning may not be necessary to achieve a good set of candidate trajectories. 

\subsection{Comparison of risk tolerance schedules}
\label{sec:betaschedule}
\begin{figure}
\centering
    \begin{subfigure}{0.45\textwidth}
        \includegraphics[width=\textwidth]{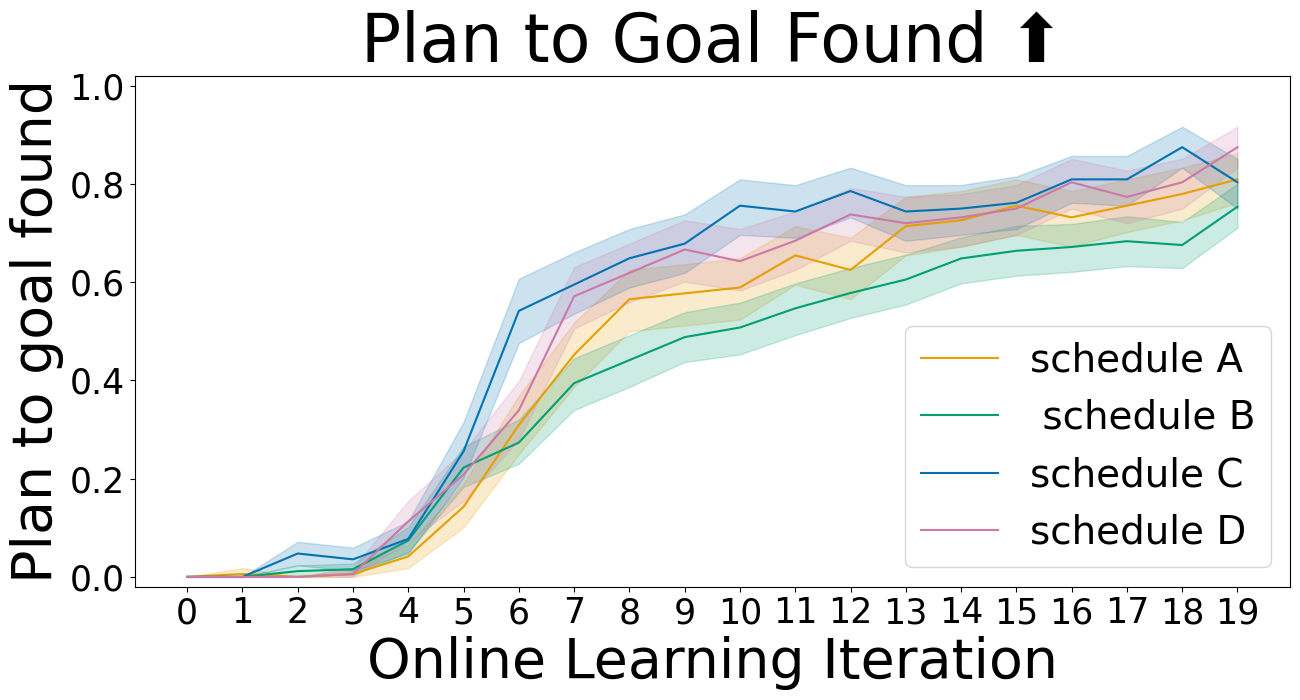} 
        \caption{Success rate in computing plans to the goal}
    \end{subfigure}
    \begin{subfigure}{0.45\textwidth}
        \includegraphics[width=\textwidth]{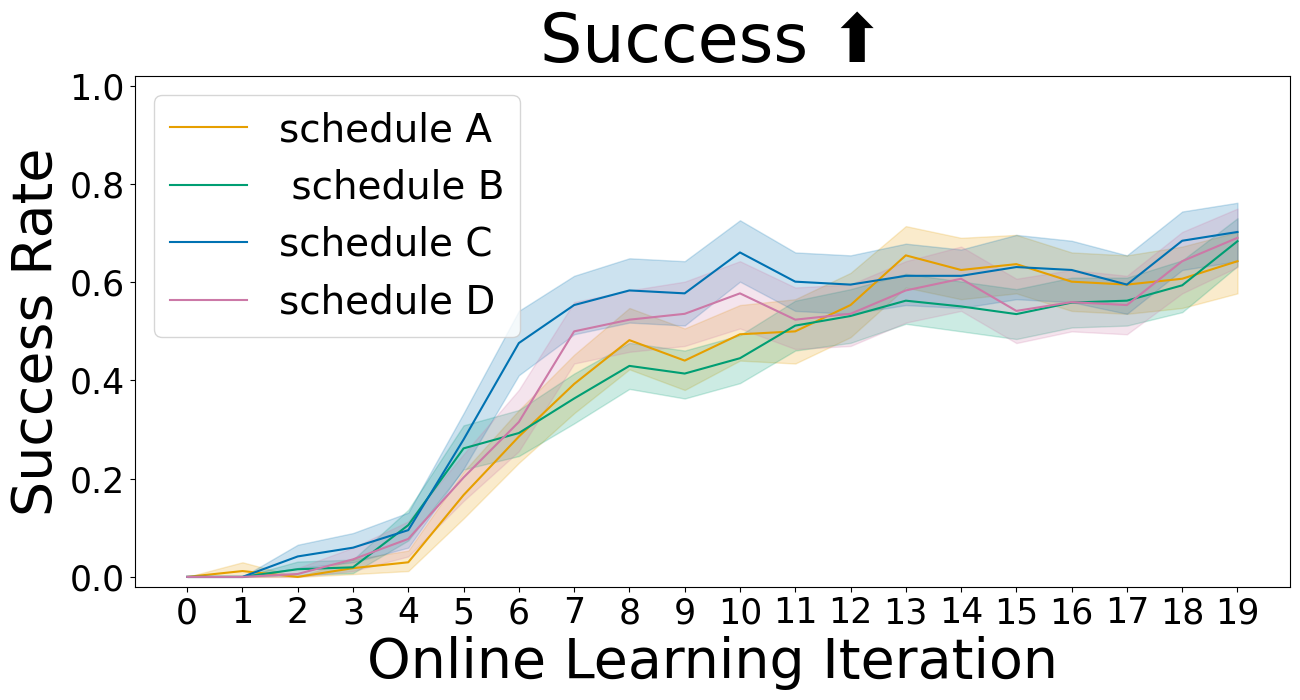} 
        \caption{Success rate in reaching the goal}
    \end{subfigure}
\caption{Effect of risk tolerance schedules on test performance. Schedule A varies $\beta$ from -2 to 2 using a sigmoid function. Schedule B is the same as schedule A, but with a maximum at 1. Schedule C fixes $\beta = -2$ and schedule D fixes $\beta=1$} 
\end{figure}

Although our acquisition function can bias data collection to low-deviation trajectories given enough data, the random generation process of RRT may not provide a sufficient set. Constraining the trajectories using the MDE during \emph{training} can improve the selection. We empirically evaluate the effect of four different beta schedules, two of which are fixed, and two of which start permissive and become more conservative. When evaluated in the simulated plant-watering domain, we observed no significant performance difference between using these schedules.
